# Supplementary material for: Spin-orbital mixing in the topological ladder of the two-dimensional metal PtTe$_2$
Source: arXiv:2502.10865 source file (2025-02-15)
Supplement: Supplementary file 1 [file PtTe2_Supplement.pdf]

# SUPPLEMENTARY INFORMATION: Spin-orbital mixing in the topological ladder of the two-dimensional metal PtTe<sub>2</sub>

M. Qahosh,<sup>1</sup> Muthu Masilamani,<sup>2,3</sup> H. Boban,<sup>1</sup> Xiao Hou,<sup>1</sup> G. Bihlmayer,<sup>4</sup> Y. Mokrousov,<sup>4</sup> W. Karain,<sup>5</sup> Jan Minár,<sup>2</sup> F. Reinert,<sup>3</sup> Jakub Schusser,<sup>2,3</sup> Claus M. Schneider,<sup>1,6,7</sup> and L. Plucinski<sup>1,8,\*</sup>

<sup>1</sup>*Peter Grünberg Institut (PGI-6), Forschungszentrum Jülich GmbH, 52428 Jülich, Germany*

<sup>2</sup>*New Technologies-Research Center, University of West Bohemia, 30614 Pilsen, Czech Republic*

<sup>3</sup>*Experimentelle Physik VII and Würzburg-Dresden Cluster of Excellence ct.qmat, Universität Würzburg, Würzburg, Germany*

<sup>4</sup>*Peter Grünberg Institut (PGI-1), Forschungszentrum Jülich and JARA, 52428 Jülich, Germany*

<sup>5</sup>*Department of Physics, Birzeit University, PO Box 14, Birzeit, Palestine*

<sup>6</sup>*Fakultät für Physik, Universität Duisburg-Essen, 47048 Duisburg, Germany*

<sup>7</sup>*Physics Department, University of California, Davis, CA 95616, USA*

<sup>8</sup>*Institute for Experimental Physics II B, RWTH Aachen University, 52074 Aachen, Germany*

(Dated: February 15, 2025)

## SI. EXPERIMENTAL METHODS

Three-dimensional spin-polarized momentum imaging has been performed using MB Scientific A1 hemispherical electron analyzer coupled with the exchange-scattering Focus GmbH FERRUM spin detector [1]. The mechano-electrostatic lens deflector system of A1 allows for mapping the emission angle over approximately  $\pm 15^\circ$  in both  $k_x$  and  $k_y$  directions, enabling point-by-point  $E_{kin}$  vs.  $k_x$  vs.  $k_y$  mapping in the spin-polarized mode without rotating the sample. All presented measurements were carried out at room temperature, providing the stability necessary for the time consuming spin measurements. As a light source we used Focus HIS 13 discharge lamp with refocussing mirror, that provided unpolarized HeI radiation ( $h\nu = 21.22$  eV) with a beam spot of size of  $< 0.5$  mm diameter. To reduce (non-significant) photon flux intensity fluctuations, the magnetization direction of the scattering target was switched at each new  $k_x$  point in reciprocal space, while filtering the in-plane  $S_y$  spin component. The measured spin polarization  $P$  is defined as  $P = \frac{A}{S}$ , where  $S$  is the Sherman function, and  $A$  is the intensity asymmetry for different magnetization directions of the scattering target. This asymmetry  $A$  for the in-plane filtered  $S_y$  spin component is defined as  $A = (I_y^{up} - I_y^{dn}) / (I_y^{up} + I_y^{dn})$ . The base pressure in the analysis chamber is  $< 5 \cdot 10^{-11}$  mbar, and rises to  $\approx 5 \cdot 10^{-9}$  mbar when using the He lamp. PtTe<sub>2</sub> sample, purchased from *HQ graphene*, was glued to the molybdenum sample plate using a silver-epoxy and cleaved using the scotch tape within the UHV system. No degradation of the PtTe<sub>2</sub> surface has been observed in our ARPES spectra within a week or more after cleavage.

In the Ferrum spin detector the oxidized Fe(001) target is rotated at  $15^\circ$  with respect to the incident electron beam [1]. In our reference frame (Figs. 1(a), 2(a), 3(a) of the main text) the target surface is rotated  $15^\circ$  around  $y$  away from the  $yz$  plane. Ferrum can probe spin polarization along 2 orthogonal quantization axes, depending

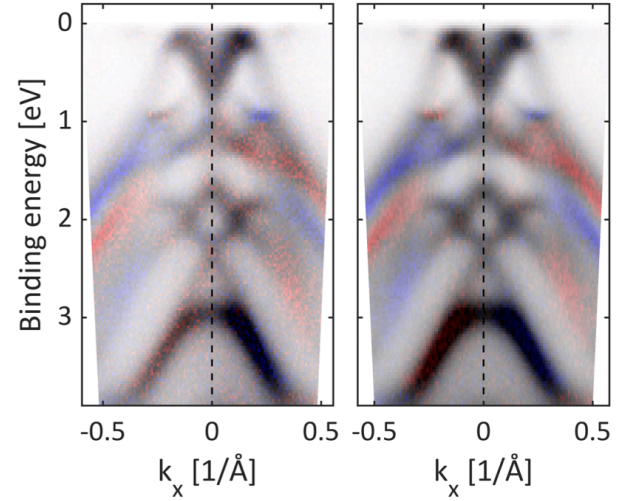

FIG. S1. Comparison of the uncorrected experimental SARPES map (left) with quantization axis at  $15^\circ$  away from the  $z$ -axis, and the corrected map (right, same as in the main text Fig. 1(g)) for the  $S_z$  quantization axis. Measurements were performed in the geometry of Fig. 1(a) of the main text.

on the target film magnetization [1]. This means that in a normal emission geometry, used for all the presented experimental data, we are probing  $S_y$  component, and a component that is  $15^\circ$  away from the  $z$  axis, which is primarily  $S_z$ , but with small component of  $S_x$ .

In the geometry in Fig. 1(a) of the main text an  $\mathcal{M}_x$  mirror plane is conserved for the experimental setup. Through the  $\mathcal{M}_x$  axial vector reflection rules this means that  $S_x(k_x, k_y, E_B) = S_x(-k_x, k_y, E_B)$  and  $S_z(k_x, k_y, E_B) = -S_z(-k_x, k_y, E_B)$ . These conditions allow, through elementary algebra, to calculate  $S_z$  maps, presented in Fig. 1(g) from the map measured at quantization axis rotated by  $15^\circ$ . Figure S1 shows the uncorrected and corrected maps.

\* l.plucinski@fz-juelich.de

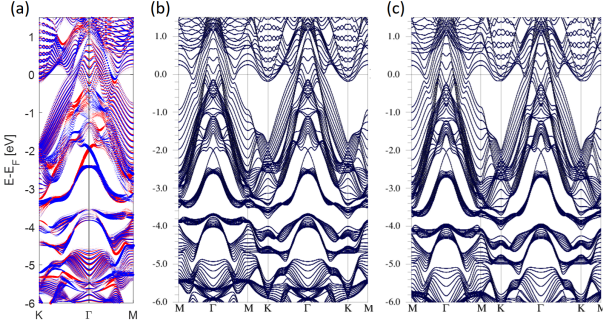

FIG. S2. Comparison of slab calculations performed at different lattice parameters, (a) Theoretically relaxed atomic positions, (b) Ref. [2], (c) Ref. [3]. Surfaces were modeled by truncated bulk lattice with 40 a.u. of vacuum. (a) was calculated using FLEUR [4] using 17L slab, (b) and (c) were calculated using WIEN2k [5] with 10L slab.

### SII. BAND STRUCTURE CALCULATIONS

Calculations shown in the main text were performed using the WIEN2k [5] in a periodic slab geometry, with 30 layers of  $\text{PtTe}_2$  (that is 90 atoms in total) separated by 40 a.u. of vacuum. In these calculations, surfaces were modeled by a truncated bulk structure (atomic positions were not relaxed). Muffin tin radius of Pt was 2.5 a.u. and of Te 2.48 a.u. Energy cutoff between valence and core electrons was set to 0.99 Ry, otherwise default WIEN2k [5] settings were used. We used lattice parameters from Ref. [2].

Additional calculations were performed using the FLEUR [4] in thin film geometry [6] choosing the generalized gradient approximation as given in Ref. [7]. The muffin-tin radii were 2.45 a.u. for Pt and Te, the product of the muffin-tin radius and the wave-function cutoff,  $RK_{\text{max}}$  was 9.31 and a  $9 \times 9$   $k$ -mesh was employed. Results using a 17 layer film in the relaxed lattice constant and including relaxations of the top three  $\text{PtTe}_2$  layers are shown in Fig. S2 (a). Comparing them to WIEN2k calculations at various lattice constants, shown in Fig. S2 (b-c) reveals no significant differences in band dispersions other than in the bandwidth.

For the calculations of fat bands shown in the main text figures we used the QTL program integrated with WIEN2k [5]. Spin polarizations, indicated by blue-red false color in theoretical band structure panels, were calculated as  $(C_{\uparrow} - C_{\downarrow}) / (C_{\uparrow} + C_{\downarrow})$ , where  $C_{\uparrow\downarrow}$  are spin up/down partial charges for the selected atomic sites and orbitals for the selected quantization axis (they take into account only charges inside the muffin tin spheres). Thickness of the "fat-bands" is proportional to  $C_{\uparrow} + C_{\downarrow}$ .

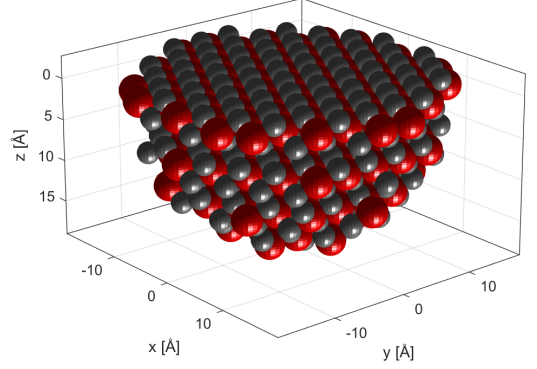

FIG. S3. Visualization of the cluster used in EDAC [8] calculations. Grey balls represent Te and red balls Pt atoms, respectively. See text for details.

### SIII. PHOTOELECTRON DIFFRACTION CALCULATIONS

Photoelectron diffraction calculations with SOC scattering have been performed using the EDAC code [8].  $\text{PtTe}_2$  surface has been simulated by the spherical cluster centered on one of the surface-most Pt atoms, with the radius of 18 Å and containing 574 atoms. The cluster is illustrated in Fig. S3. The inelastic mean free path of 3 Å and inner potential of  $V_0 = 15$  eV have been used.

We used the same lattice parameters as for the band structure calculations. Two separate calculations for the initial  $s$ -wave spin polarized up to down along the  $y$ -axis were performed, this initial emission can be written as  $S_{i\uparrow}(\theta, \phi)$  and  $S_{i\downarrow}(\theta, \phi)$  which are just fully isotropic spin polarized waves emitted from Pt site. This is needed to obtain results from non-spin-polarized initial state. Subsequently, in both cases, the final state spin polarization along  $y$ -axis was calculated, therefore obtaining 2 multiply scattered wave functions  $S_{i\uparrow, f\uparrow}(\theta, \phi)$ , and  $S_{i\downarrow, f\downarrow}(\theta, \phi)$ . In order to obtain intensities shown in Fig. 4 (d)-(e) of the main text, we calculated  $I_{\uparrow} = |S_{i\uparrow, f\uparrow}(\theta, \phi)|^2$  and  $I_{\downarrow} = |S_{i\downarrow, f\downarrow}(\theta, \phi)|^2$ .

### SIV. ONE-STEP MODEL CALCULATIONS

The SARPES spectra are calculated using multiple-scattering Green's function formalism within the Spin-Polarised Relativistic Korringa-Kohn-Rostoker (SPR-KKR) band structure package [9]. The photoemission (PE) calculations are based on the one-step PE model and spin density matrix formulations of the multiple scattering operator to calculate the photocurrent, resulting in a good description of the underlying PE phenomena related to the matrix element [10, 11]. The spin-orbit

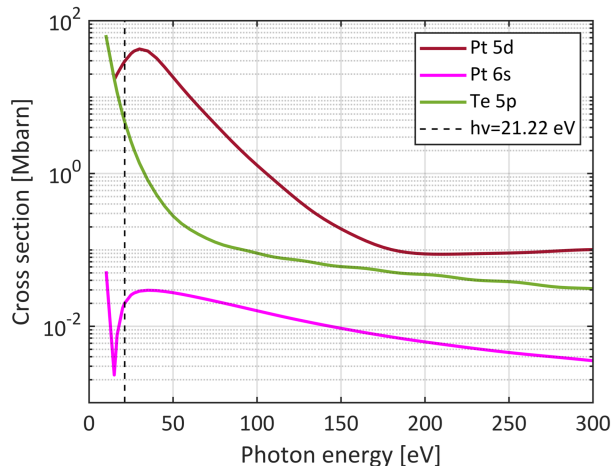

FIG. S4. Photoionization cross sections for relevant Pt and Te orbitals [16]. Dashed vertical line indicates  $h\nu = 21.2$  at which experiments were performed.

coupling (SOC) is considered via solving a fully relativistic Dirac equation [12]. We employed full-potential approximations to accurately describe the self-consistent potential variations [13]. We used Rundgren-Malmström (RM) model surface barrier potential and the selfconsistently calculated crystal potential for a reliable description of the initial and final states [14]. The initial and final wavefields and their derivatives must be continuous at the boundary between surface and bulk. This boundary is defined by the so-called image plane and its position along the  $z$ -axis allows the modification of the shape of the RM potential  $VB(z)$ . The surface barrier potential asymptotically connects the bulk potential to the vacuum. In our calculations, we used RM type of barrier to

simulate the potential gradient at the front of the surface layer [15]. The convergence of multiple scattering between layers in the semi-infinite crystal was reached with 125 reciprocal lattice  $g$ -vectors in the plane wave basis representation. While solving the Dyson equation within the multiple scattering Green's function formalism, we use Bauer's identity to represent the scattering between and inside the layers as plane and spherical wavefield, respectively. The summation involved in the expansion of these waves in angular momentum basis was limited at  $l_{max} = 4$ . The lifetime of initial and final states was simulated using the imaginary part of  $V_{0i} = 5$  meV and  $V_{0f} = 1$  eV of the potential, respectively. Both time-reversed LEED and free-electron final states by the design of the layered KKR formalism contain the damping induced by the  $V_{0f}$ . SRP-KKR map in Fig. 1 (g) of the main text has been symmetrized as  $S_y(k_x) = -S_y(-k_x)$  to account for the minor numerical asymmetries.

## SV. PHOTOIONIZATION CROSS-SECTIONS

Figure S4 shows photoionization cross sections [16] (see also WebElements at [vuo.elettra.eu](http://vuo.elettra.eu)) for the relevant valence orbitals of  $PtTe_2$ . One can see that at  $h\nu = 21.2$  eV Pt  $5d$  and Te  $5p$  dominate, with the cross section ratio of  $\approx 3/1$ . Taking into account short mean free part at experimental kinetic energies (inside the solid) of around 17 – 21 eV, the contributions from the surface most Te1 and Pt atoms (see Figs. 1 (i) and 4 (a) of the main text) are probably similar. This means that at least both Te1 and Pt sites should be taken into account in the analysis of the SARPES signal, with an additional minor contribution from Te2. Deeper sites will also contribute, but not significantly, however indications of  $k_z$  dispersion suggest that their contribution might be non-negligible.

- [1] M. Escher, N. B. Weber, M. Merkel, L. Plucinski, and C. M. Schneider, *e-Journal of Surface Science and Nanotechnology* **9**, 340–343 (2011).
- [2] TheMaterialsProject [10.17188/1207707](https://doi.org/10.17188/1207707) (2020).
- [3] *PtTe<sub>2</sub> Crystal Structure: Datasheet from “PAULING FILE Multinaries Edition – 2022” in SpringerMaterials*, publisher=“Springer-Verlag Berlin Heidelberg & Material Phases Data System (MPDS), Switzerland & National Institute for Materials Science (NIMS), Japan, copyright 2023 Springer-Verlag Berlin Heidelberg & Material Phases Data System (MPDS), Switzerland & National Institute for Materials Science (NIMS), Japan.
- [4] D. Wortmann, G. Michalick, N. Baadji, M. Betzinger, G. Bihlmayer, J. Bröder, T. Burnus, J. Enkovaara, F. Freimuth, C. Friedrich, C.-R. Gerhorst, S. Granberg Cauchi, U. Grytsiuk, A. Hanke, J.-P. Hanke, M. Heide, S. Heinze, R. Hilgers, H. Janssen, D. A. Klüppelberg, R. Kovacik, P. Kurz, M. Lezaic, G. K. H. Madsen, Y. Mokrousov, A. Neukirchen, M. Redies, S. Rost, M. Schlupf, A. Schindlmayr, M. Winkelmann, and S. Blügel, *FLEUR*, Zenodo

- <https://doi.org/10.5281/zenodo.7576163> (2023).
- [5] P. Blaha, K. Schwarz, F. Tran, R. Laskowski, G. K. H. Madsen, and L. D. Marks, *The Journal of Chemical Physics* **152**, 074101 (2020), <https://pubs.aip.org/aip/jcp/article-pdf/doi/10.1063/1.5143061/16727313/074101.1.online.pdf>.
- [6] H. Krakauer, M. Posternak, and A. J. Freeman, *Phys. Rev. B* **19**, 1706 (1979).
- [7] J. P. Perdew, K. Burke, and M. Ernzerhof, *Physical Review Letters* **77**, 3865 (1996).
- [8] F. J. García de Abajo, M. A. Van Hove, and C. S. Fadley, *Phys. Rev. B* **63**, 075404 (2001).
- [9] H. Ebert, D. Ködderitzsch, and J. Minár, *Reports on Progress in Physics* **74**, 096501 (2011).
- [10] J. Pendry, *Surface Science* **57**, 679 (1976).
- [11] J. Braun, *Reports on Progress in Physics* **59**, 1267 (1996).
- [12] J. Braun, J. Minár, and H. Ebert, *Physics Reports* **740**, 1 (2018), correlation, temperature and disorder: Recent developments in the one-step description of angle-resolved photoemission.

- [13] V. N. Strocov, L. L. Lev, F. Alarab, P. Constantinou, X. Wang, T. Schmitt, T. J. Z. Stock, L. Nicolăi, J. Očenášek, and J. Minár, *Nature Communications* **14**, 10.1038/s41467-023-40432-5 (2023).
- [14] G. Malmström and J. Rundgren, *Computer Physics Communications* **19**, 263 (1980).
- [15] M. Masilamani, J. Schusser, M. Qahosh, L. Plucinski, and F. Reinert, *AIP Conference Proceedings* **3054**, 070004 (2024), [https://pubs.aip.org/aip/acp/article-pdf/doi/10.1063/5.0187969/18572678/070004\\_1\\_5.0187969.pdf](https://pubs.aip.org/aip/acp/article-pdf/doi/10.1063/5.0187969/18572678/070004_1_5.0187969.pdf).
- [16] J. Yeh and I. Lindau, *Atomic Data and Nuclear Data Tables* **32**, 1 (1985).
